# Supplementary material for: Memory-constrained Vectorization and Scheduling of Dataflow Graphs for Hybrid CPU-GPU Platforms
Source: arXiv:1711.11154 source file (2017-11-29)
Supplement: Supplementary file 1 [file appendix.tex]

\appendix
\section {Theorems and Proofs}
\subsection{Vectorization Degrees}
\subsection{Throughput of Vectorized SDF}
\label{sec:apdx-th}
